# Supplementary material for: On Evaluating Adversarial Robustness of Volumetric Medical Segmentation Models
Source: arXiv:2406.08486 source file (2024-09-02)
Supplement: Supplementary file 1 [file bmvc_appendix.tex]

\documentclass{bmvc2k}

\usepackage{multirow}
\usepackage{booktabs}       % professional-quality tables
\usepackage{color}
\usepackage{colortbl}
\usepackage{graphicx} 
\usepackage{diagbox}

\definecolor{Gray}{gray}{0.90}
\definecolor{white}{rgb}{1.0, 1.0, 1.0}

\definecolor{LightCyan}{RGB}{240, 224, 238}
% \newcolumntype{a}{>{\columncolor{LightCyan}}c}

%% Enter your paper number here for the review copy
\bmvcreviewcopy{681}

\title{Adversarial Robustness Comparison of CNN, Transformer and Mamba-based Medical Segmentation Models}

% Enter the paper's authors in order
% \addauthor{Name}{email/homepage}{INSTITUTION_CODE}
\addauthor{Susan Student}{http://www.vision.inst.ac.uk/~ss}{1}
\addauthor{Petra Prof}{http://www.vision.inst.ac.uk/~pp}{1}
\addauthor{Colin Collaborator}{colin@collaborators.com}{2}

% Enter the institutions
% \addinstitution{Name\\Address}
\addinstitution{
 The Vision Institute\\
 University of Borsetshire\\
 Wimbleham, UK
}
\addinstitution{
 Collaborators, Inc.\\
 123 Park Avenue,\\
 New York, USA
}

\runninghead{Student, Prof, Collaborator}{BMVC Author Guidelines}

% Any macro definitions you would like to include
% These are not defined in the style file, because they don't begin
% with \bmva, so they might conflict with the user's own macros.
% The \bmvaOneDot macro adds a full stop unless there is one in the
% text already.

% New Packages
\usepackage{amsmath,amsfonts,amssymb}

%-------------------------------------------------------------------------

\begin{document}

\maketitle

%-------------------------------------------------------------------------

\newpage
\bibliography{egbib}

\end{document}
